# Supplementary material for: Supersymmetric polarization anomaly in photonic discrete-time quantum walks
Source: arXiv:1804.09496 source file (2019-01-18)
Supplement: Supplementary file 1 [file SuppMat_PRL.pdf]

# Supplemental Material: Supersymmetric polarization anomaly in photonic discrete-time quantum walks

## SUPPLEMENTAL FIGURES

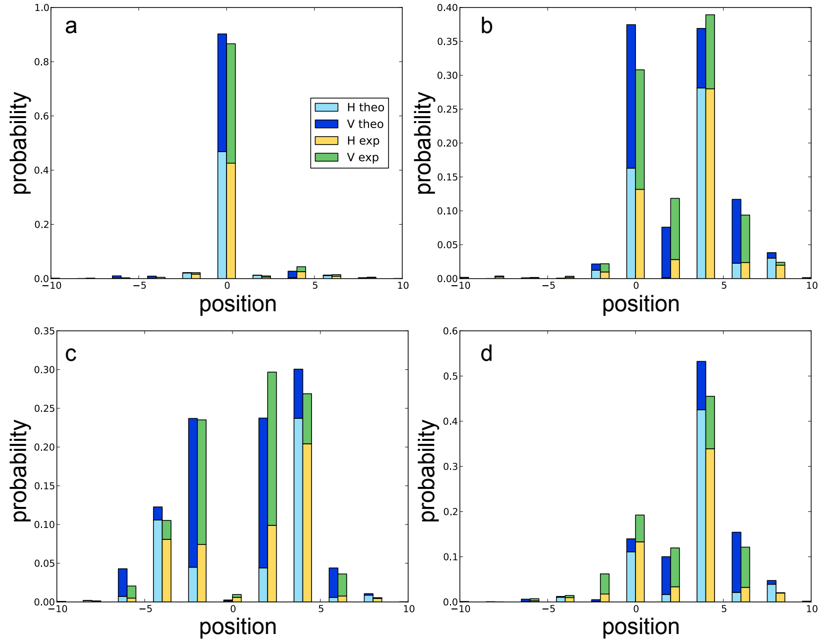


FIG. S1. Intensity histogramms for step 17 for the interface configuration (a,b) and interface-free bulk system (c,d) complementing Fig. 3 in the main text. The input polarizations are $|H\rangle$ (a,c) and $C_{\mathrm{QWP}}(137°)|H\rangle = 0.72|H\rangle + (0.12 + i0.69)|V\rangle$ (b,d). Experimental results (orange, light blue) are compared to numerical simulations (red, dark blue) of the quantum walk with the specified Floquet operator in the H′/ V′ timeframe. (a) A strong trapping at the interface at $x = 0$ is observed. As predicted the intensities of the H and the V light are almost equally strong. (b) For a non-perfect overlapping input polarization the trapping at $x = 0$ is less dominant, but still discernible. Again the H and V intensities at $x = 0$ have similar heights. (c),(d) In absence of the midgap state, no significant trapping occurs for neither input polarization.

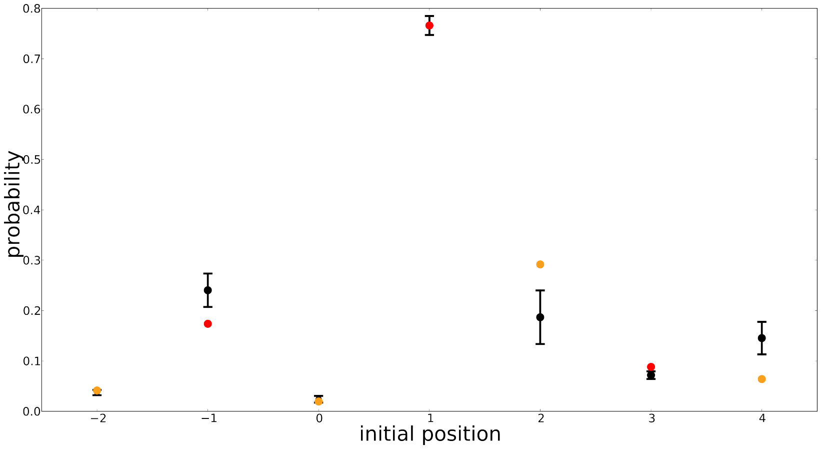


FIG. S2. Dependence of the trapped light intensity on the in-coupling position, measured after 13 steps at the defect position in the interface configuration. The initial polarization is $|H\rangle$. Black symbols including error bars denote the experimental data while the dots give the results of the numerical simulations. Depending on the initial position, the readout is at $x = 0$ (red dots) or $x = 1$ (orange dots). We observe the expected intensity decay when the spatial overlap between the initial and the midgap state is reduced, the overlap in polarization is constant in this setting.

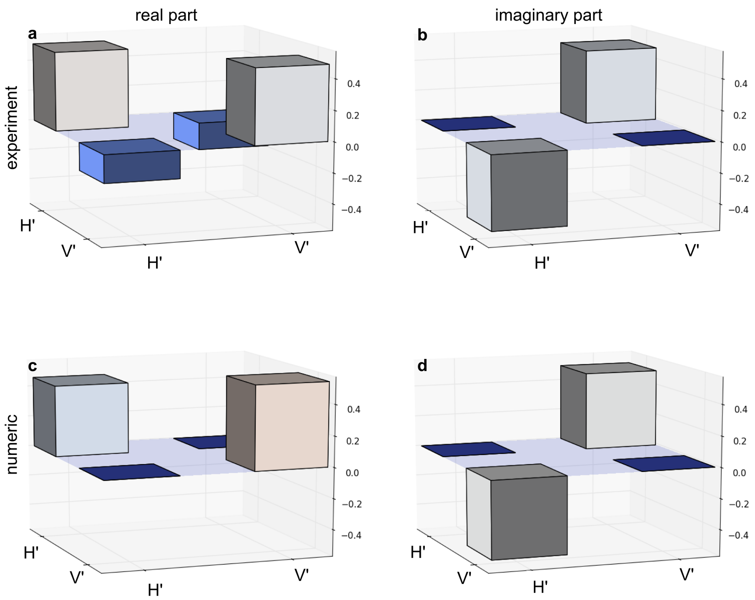


FIG. S3. **Anomalous polarization of the trapped midgap state** from tomography of the polarization state at $x = 1$ (same configuration as in Fig. 3 in the main text, but measured one step earlier, i.e. step 16). The off-diagonal elements of the imaginary part now indicate a $-\pi/2$ phase shift between them, corresponding to left-handed polarization. From the experimental data we find the polarization state $(0.72 \pm 0.01)|H'\rangle + (0.70 \pm 0.01)\exp((-0.61 \pm 0.01)i\pi)||H\rangle'\rangle$, while numerically $0.68|H'\rangle + 0.74\exp(-0.50i\pi)|V'\rangle$.

## S1: FLOQUET-BLOCH THEORY

We employ standard Floquet-Bloch theory [S1, S2] in order to analyze the bulk configuration of the discrete-time quantum walk. The bulk realizes an infinitely periodic system made of two-site unit cells. Enumerating the cell by an index $n$, the extended states assume the dependence

$$\Psi_{2n-1,H}(t) = h_o(k)\exp(ikn - i\epsilon(k)t), \quad \Psi_{2n,H}(t) = h_e(k)\exp(ikn - i\epsilon(k)t), \tag{S1}$$

$$\Psi_{2n-1,V}(t) = v_o(k)\exp(ikn - i\epsilon(k)t), \quad \Psi_{2n,V}(t) = v_e(k)\exp(ikn - i\epsilon(k)t), \tag{S2}$$

where we collect the amplitudes at odd and even sites into a vector $\psi = (h_o, v_o, h_e, v_e)^T$. Evaluating the evolution of this state over one step delivers eq. (3), and equivalently eq. (5) in the main text, with relevant Pauli matrices

$$\sigma_x = \begin{pmatrix} 0 & 1 & 0 & 0 \\ 1 & 0 & 0 & 0 \\ 0 & 0 & 0 & 1 \\ 0 & 0 & 1 & 0 \end{pmatrix}, \quad \sigma_y = \begin{pmatrix} 0 & -i & 0 & 0 \\ i & 0 & 0 & 0 \\ 0 & 0 & 0 & -i \\ 0 & 0 & i & 0 \end{pmatrix}, \quad \Sigma_z = \begin{pmatrix} 1 & 0 & 0 & 0 \\ 0 & 1 & 0 & 0 \\ 0 & 0 & -1 & 0 \\ 0 & 0 & 0 & -1 \end{pmatrix} \tag{S3}$$

According to

$$0 = \psi^\dagger(\sigma_y u' - u'^\dagger \sigma_y)\psi = (\lambda - \lambda^{-1})\psi^\dagger \sigma_y \psi, \tag{S4}$$

Floquet-Bloch states with $\lambda \neq \pm 1$ have a vanishing expectation value $\langle \sigma_y \rangle = 0$, meaning that averaged over a unit cell they are linearly polarized in the H$'$/ V$'$ basis. Analogously,

$$0 = \psi^\dagger(\Sigma_z \sigma_y u' + u'^\dagger \Sigma_z \sigma_y)\psi = (\lambda + \lambda^{-1})\psi^\dagger \Sigma_z \sigma_y \psi, \tag{S5}$$

hence $\langle \Sigma_z \sigma_y \rangle = 0$ unless $\lambda = \pm i$, meaning that the degree of circular polarizations on each of the two sites within the unit cell must be identical. Therefore, unless a state is pinned to a symmetry-protected value of $\lambda$, its degree of circular polarization must vanish on each site, which constraints all bulk states. Combining these expectation values with

$$0 = \psi^\dagger(u'^\dagger \Sigma_z u' + \Sigma_z)\psi = 2\psi^\dagger \Sigma_z \psi, \tag{S6}$$

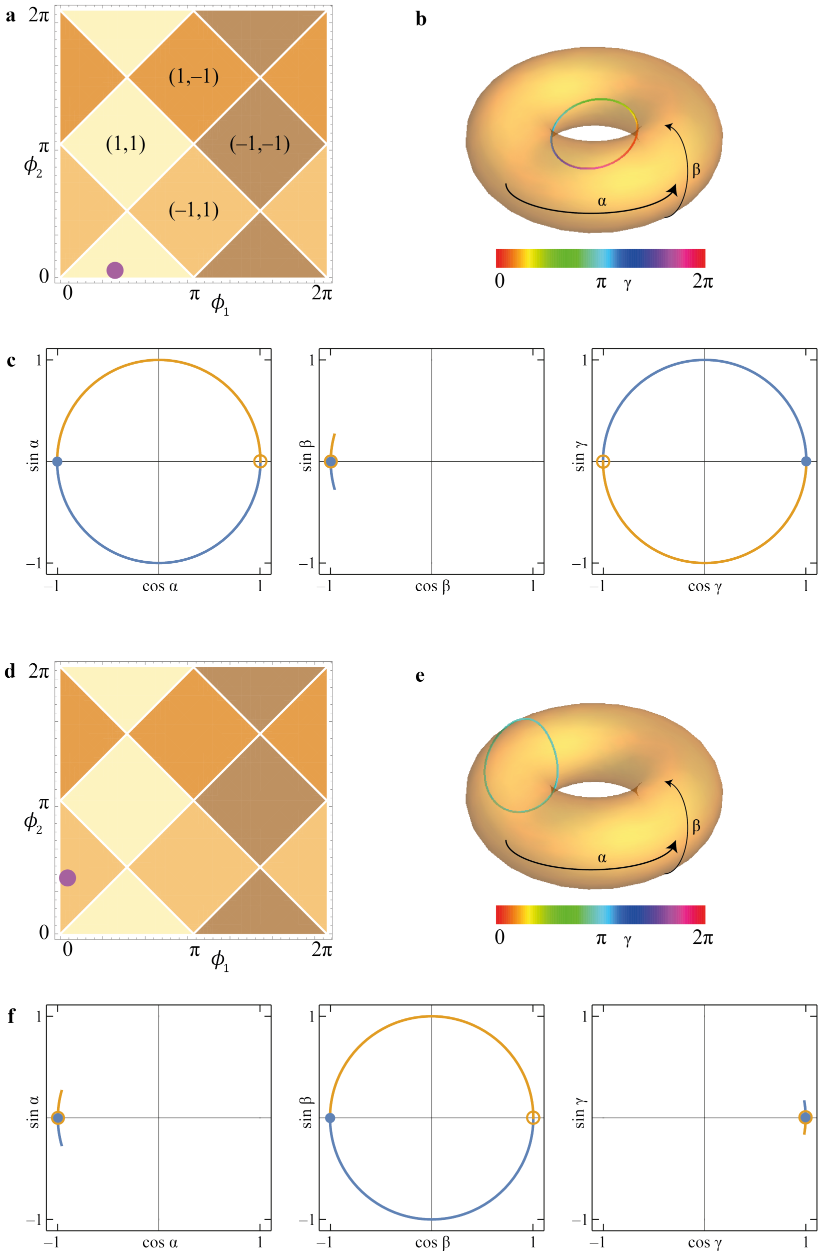


FIG. S4. Winding of the Floquet-Bloch states as one traverses the Brillouin zone. The states are parameterised by three angles $(\alpha, \beta, \gamma)$ defining a three-torus $T^3$. The two situations correspond to the two phases in the experiments, with $(\varphi_1, \varphi_2) = (1.29, 0.17)$ (a-c, representing the bulk configuration and the region $x \geq 1$ in the interface configuration), and $(\varphi_1, \varphi_2) = (0.17, 1.29)$ (d-f, representing the region $x \leq 0$ in the interface configuration). The circles in panels a,d locate these parameters in the phase space of the system, where identical colors indicate gapped regions with the same topological indices $(\nu, \nu')$. Panels b,e show the winding in a representation utilizing a two-torus for $(\alpha, \beta)$ and a periodic colour coding for $\gamma$. Panels c,f show the winding of each angle separately, where the blue dot represents the position at $k = 0$ and the orange circle the position at $k = \pi$. The blue curve traces the state over the interval $k \in (0, \pi)$, while the orange curve covers the range $k \in (\pi, 2\pi)$.

and hence $\langle \Sigma_z \rangle = 0$, the representation eq. (9) of Bloch states on the three-torus $T^3$ shown in Fig. 1d and Fig. S4(b,e) follows from their parametrization (see also Sec. S2)

$$\psi(k) = \frac{e^{i\delta}}{2\sqrt{2}} \begin{pmatrix} 1 - ie^{i\alpha} \\ -i + e^{i\alpha} \\ e^{i\gamma}(1 - ie^{i\beta}) \\ e^{i\gamma}(-i + e^{i\beta}) \end{pmatrix}. \tag{S7}$$

To determine the anomalous polarization pattern of interface states pinned to $\lambda = \pm i$, we identify the decaying evanescent waves from the condition $\mathrm{Re}[\lambda^2(k)] = \cos(\varphi_1)\cos(\varphi_2)\cos(k) - \sin(\varphi_1)\sin(\varphi_2) = 0$. In the H′/ V′ basis and up to overall normalization, these waves on the even and odd sites take the form

$$\Psi_{2n-1,H'}(t) = i\Lambda^n(\pm i)^t, \quad \Psi_{2n,H'}(t) = \mu\Lambda^n(\pm i)^t, \tag{S8}$$

$$\Psi_{2n-1,V'}(t) = \Lambda^n(\pm i)^t, \quad \Psi_{2n,V'}(t) = i\mu\Lambda^n(\pm i)^t, \tag{S9}$$

where

$$\mu = \pm\frac{\cos(\varphi_1/2) - \sin(\varphi_1/2)}{\cos(\varphi_2/2) - \sin(\varphi_2/2)} \tag{S10}$$

and

$$\Lambda = \frac{\sin((\varphi_1 - \varphi_2)/2) - \cos((\varphi_1 + \varphi_2)/2)}{\sin((\varphi_1 - \varphi_2)/2) + \cos((\varphi_1 + \varphi_2)/2)}, \tag{S11}$$

so that $\Lambda < 1$ decays to the right if $\nu = 1$, and $\Lambda > 1$ giving decay to the left if $\nu = -1$, with the topological index $\nu = \mathrm{sgn}[\cos((\varphi_1 + \varphi_2)/2)\sin((\varphi_1 - \varphi_2)/2)]$. For an interface pinning states to $\lambda = \pm 1$, an analogous application of this method delivers evanescent states of identical circular polarization on all sites, whose decay is determined by the topological index $\nu' = \mathrm{sgn}[\sin((\varphi_1 + \varphi_2)/2)\cos((\varphi_1 - \varphi_2)/2)]$. These topological indices are identical to those in the split-step partner [S1, S2] systems described by eq. (6). For our experimental choice of angles, in the interface configuration a system with $(\nu, \nu') = (-1, 1)$ is placed to the left of a system with $(\nu, \nu') = (1, 1)$. This produces midgap states confined to the interface, with a circular polarization that alternates between right-handed on even sites and left-handed on odd sites. If we alternatively had realized an interface with a region $(\nu, \nu') = (1, 1)$ is placed to the left of a system with $(\nu, \nu') = (-1, 1)$, the sense of circular polarization would be switched around.

## S2: RELATION OF THE TOPOLOGICAL INDICES TO WINDING NUMBERS

The combination of chirality and supersymmetry imply that the states in the Floquet-Bloch bands have vanishing expectation values $\langle\sigma_y\rangle = \langle\Sigma_z\sigma_y\rangle = \langle\Sigma_z\rangle = 0$. This allows to parametrize these states as

$$\psi(k) = \frac{e^{i\delta}}{2\sqrt{2}}\begin{pmatrix} 1 - ie^{i\alpha} \\ -i + e^{i\alpha} \\ e^{i\gamma}(1 - ie^{i\beta}) \\ e^{i\gamma}(-i + e^{i\beta}) \end{pmatrix}. \tag{S12}$$

where $\delta$ is a global $U(1)$ phase that we disregard, while $(\alpha, \beta, \gamma)$ define a three-torus $T^3$ that can be extracted from the expectation values

$$(\cos(\alpha), \sin(\alpha)) = (\langle\sigma_x(1 + \Sigma_z)\rangle, \langle\sigma_z(1 + \Sigma_z)\rangle), \tag{S13}$$

$$(\cos(\beta), \sin(\beta)) = (\langle\sigma_x(1 - \Sigma_z)\rangle, \langle\sigma_z(1 - \Sigma_z)\rangle), \tag{S14}$$

$$(\cos(\gamma), \sin(\gamma)) = (\langle\Sigma_x(1 - \sigma_y)\rangle, \langle\Sigma_y(1 - \sigma_y)\rangle). \tag{S15}$$

As $k$ traverses the Brillouin zone in a system with fixed $\varphi_1$ and $\varphi_2$, the states in each Floquet-Bloch band trace out closed loops around $T^3$, giving rise to three winding numbers $\nu_\alpha, \nu_\beta, \nu_\gamma$. Since the four bands are connected via multiplications of the states with $\sigma_y, \Sigma_z\sigma_y$, and $\Sigma_z$ that correspond to rotations of these loops, the winding numbers are the same for all four bands. These winding numbers can only change when a gap closes. They can therefore be inferred from any combination of $\varphi_1$ and $\varphi_2$ within a gapped phase, for which we choose points of high symmetry. The combinations below exhaust all gapped phases (see Fig. S4a), within which they identify central points with flat bands pinned to $\lambda = \pm\sqrt{\pm i}$. For each case, we provide the parametrization of the flat band pinned to $\lambda = \sqrt{i}$ in the first quadrant of the $\lambda$ plane:

| $(\varphi_1,\varphi_2)$ | $(\nu,\nu')$ | $(\alpha,\beta,\gamma)(k)$ | $(\nu_\alpha,\nu_\beta,\nu_\gamma)$ |
|---|---|---|---|
| $(\pi/2,0)$ | $(1,1)$ | $(k+\pi,\pi,k)$ | $(1,0,1)$ |
| $(\pi/2,\pi)$ | $(1,1)$ | $(k,0,k+\pi)$ | $(1,0,1)$ |
| $(3\pi/2,0)$ | $(-1,-1)$ | $(-k,0,\pi)$ | $(-1,0,0)$ |
| $(3\pi/2,\pi)$ | $(-1,-1)$ | $(-k+\pi,\pi,\pi)$ | $(-1,0,0)$ |
| $(0,\pi/2)$ | $(-1,1)$ | $(\pi,k+\pi,0)$ | $(0,1,0)$ |
| $(\pi,\pi/2)$ | $(-1,1)$ | $(0,k,\pi)$ | $(0,1,0)$ |
| $(0,3\pi/2)$ | $(1,-1)$ | $(0,-k,k+\pi)$ | $(0,-1,1)$ |
| $(\pi,3\pi/2)$ | $(1,-1)$ | $(\pi,-k+\pi,k+\pi)$ | $(0,-1,1)$ |

Therefore,

$$\nu_\alpha=\frac{\nu+\nu'}{2},\quad \nu_\beta=\frac{-\nu+\nu'}{2},\quad \nu_\gamma=\frac{\nu+1}{2}, \tag{S16}$$

so that in our system only two winding numbers are independent. This constraint arises from time-reversal symmetry, $[u''(k)]^T=u''(k)$ with $u''(k)=\exp(-\Sigma_z k/2)u'\exp(i\Sigma_z k/2)$, so that in the basis of $u''(k)$ all eigenvectors can be written as real but pick up an extra phase $\pi$ as one transverses the Brillouin zone. In the original basis this implies $\nu_\gamma+(\nu_\beta-\nu_\alpha)/2=1/2$. In the experiments, we couple a system with indices $(\nu,\nu')=(-1,1)$ and winding numbers $(\nu_\alpha,\nu_\beta,\nu_\gamma)=(0,1,0)$ to a system with indices $(\nu,\nu')=(1,1)$ and winding numbers $(\nu_\alpha,\nu_\beta,\nu_\gamma)=(1,0,1)$. These windings are illustrated in Fig. S4.

## S3: EXPERIMENTAL SETUP

The laser used in the experiment is a diode laser with a central wavelength of 805 nm. It produces pulses of approximately 88 ps FWHM duration and a variable repetition rate, chosen with respect to the duration of a full quantum walk. The input quarter or half waveplate (QWP, HWP) can generate a variably polarized input state via the transformations

$$C_{\text{QWP}}(\alpha)=\frac{-i}{\sqrt{2}}\begin{pmatrix}\cos(2\alpha)+i & \sin(2\alpha)\\ \sin(2\alpha) & -\cos(2\alpha)+i\end{pmatrix}, \tag{S17}$$

$$C_{\text{HWP}}(\alpha)=\begin{pmatrix}\cos(2\alpha) & \sin(2\alpha)\\ \sin(2\alpha) & -\cos(2\alpha)\end{pmatrix}. \tag{S18}$$

A Soleil-Babinet compensator (SBC) and electro-optic modulator (EOM) [S3–S6] realise the dynamic coin operation in the H/V basis according to the matrix (2) in the main text. The EOM is controlled by applying a voltage $U$, which can be dynamically switched between three values $-U_0,0,U_0$ corresponding to rotation angles $-\varphi_{\text{EOM}},0,\varphi_{\text{EOM}}$. The SBC provides a static offset angle $\varphi_{\text{SBC}}$ based on the same transformation matrix, yielding in combination three dynamically selectable coin operations $-\varphi_{\text{EOM}}+\varphi_{\text{SBC}},\varphi_{\text{SBC}},\varphi_{\text{EOM}}+\varphi_{\text{SBC}}$. A particular coin distribution can be achieved by appropriately programming the switching times and rotation angles of the EOM to address the corresponding pulses. To realise the partial shift in the step operation, two single-mode fibres of 448 m and 470 m length have been used leading to a position separation of 110 ns and a step separation of 2.22 $\mu$s. The detectors measuring the outcoupled signal are silicon-based avalanche photo diodes operating in Geiger mode with a dead time of about 50 ns and detection efficiencies around 65%.

Quarter or half wave plates in front of the detection unit perform the basis transformations to the different measurement bases for the polarization tomography [S5–S8]. We measure the full polarization state of the walker after 16 and 17 steps on site $x=1$ and $x=0$, respectively, in the horizontal-vertical, diagonal-antidiagonal and right and left-hand circular bases. From this set of measurements we extract the Stokes parameters $S_i$ and calculate the density-matrix via $\rho=\frac{1}{2}\Sigma_{i=0)}^{3}S_i\sigma_i$. The polarization state $a|H\rangle+b\exp(i\chi)|V\rangle$ with real $a,b,\chi$ in the experimental H/V basis follows from comparison with $\rho=\begin{pmatrix}a^2 & ab\exp(-i\chi)\\ ab\exp(i\chi) & b^2\end{pmatrix}$, and its transformation to the symmetric H′/V′ basis follows from eq. (6), as shown in Figs. 3 and S3.

## S4: EXPERIMENTAL ERRORS AND NUMERICAL SIMULATIONS

We have identified three sources of systematic errors to define a realistic model of our experiment: first, the efficiencies of the two detectors, which were determined in a separate measurement and for which the measurement data is corrected; second, the different losses experienced in different paths due to dissimilar coupling efficiencies and path geometries, which were similarly estimated in an independent measurement with an accuracy of $\pm 1.5\%$; third, the angles of the EOM, the SBC and the input QWP and HWP, which can be set only with a precision of $\pm 1^{\circ}$. For the determination of the coupling efficiencies and all angles, we resorted to a numerical model. In a Monte Carlo simulation, we randomly chose 1000 sets from the parameters within the identified ranges. The set yielding the best reproduction of the experimental data (we calculated the distance between simulation and experiment for the first seven round trips) was chosen for a realistic model. The standard deviation of the statistics produced by the Monte Carlo simulation from the realistic model determines the size of the presented errors, e.g. shown in Figs. 2e (main text) and S2. These errors are then propagated to identify the uncertainties of the reconstructed polarization state in Fig. 3 (main text). In order to achieve a good signal-to-noise ratio for high step numbers presented in the main text we take measurements with two different initial power levels, which are then concatenated for the chessboard patterns showing the intensity evolution. This concatenation of two data sets is necessary since for a low power input the signal becomes to small after nine steps, while the high input powers cause detector saturation for the early steps and make a reliable probability extraction for steps one to five impossible.


[S1] T. Kitagawa, M. S. Rudner, E. Berg, and E. Demler, Physical Review A **82**, 033429 (2010).

[S2] J. K. Asbóth, Physical Review B **86**, 195414 (2012).

[S3] A. Schreiber, K. N. Cassemiro, V. Potoček, A. Gábris, I. Jex, and C. Silberhorn, Physical Review Letters **106**, 180403 (2011).

[S4] A. Schreiber, A. Gábris, P. P. Rohde, K. Laiho, M. Štefaňák, V. Potoček, C. Hamilton, I. Jex, and C. Silberhorn, Science **336**, 55 (2012).

[S5] F. Elster, S. Barkhofen, T. Nitsche, J. Novotný, A. Gábris, I. Jex, and C. Silberhorn, Scientific Reports **5**, 13495 (2015).

[S6] T. Nitsche, F. Elster, J. Novotný, A. Gábris, I. Jex, S. Barkhofen, and Christine Silberhorn, New Journal of Physics **18**, 063017 (2016).

[S7] D. F. V. James, P. G. Kwiat, W. J. Munro, and A. G. White, Physical Review A **64**, 052312 (2001).

[S8] S. Barkhofen, T. Nitsche, F. Elster, L. Lorz, A. Gábris, I. Jex, and C. Silberhorn, Physical Review A **96**, 033846 (2017).
